# Supplementary material for: Hand-breathe: Non-Contact Monitoring of Breathing Abnormalities from Hand Palm
Source: arXiv:2212.06089 source file (2022-12-12)
Supplement: Supplementary file 1 [file appendix.tex]

\section{}
